# Supplementary material for: Retrieval Based Time Series Forecasting
Source: arXiv:2209.13525 source file (2022-09-27)
Supplement: Supplementary file 1 [file 08_appendix.tex]

\section{Implementation Details}
% The retrieval model and the generation model are implemented separately.
For the retrieval model, we set the damping factor of RWR as $c=0.9$.
Given a target time series snippet, which starts from the time $T_S$ and ends at the time $T_E$, for imputation, the time span of the references is also from $T_S$ to $T_E$; 
for forecasting, we use reference snippets from a prior time, and the time span of the references is from $T_S-\Delta T$ to $T_E-\Delta T$, where $\Delta T$ is the time shift.
For traffic/temperature/revenue, $\Delta T$ is one week/one year/two years respectively.
For networked time series forecasting, given a target time series, we allow the retrieval model to retrieve its own historical snippets as references.

The implementation details of the generation model are presented below.
The hidden dimensions for the traffic/temperature/revenue datasets are 256/64/64. 
The numbers of blocks and attention heads are 8 and 4.
We use Adam optimizer \cite{kingma2014adam} to train models, and the learning rates are tuned within [0.001, 0.0001].
Early stopping is applied on the validation set to prevent over-fitting.
The patience of early stopping is set as 10.
The model is implemented by PyTorch (\url{https://pytorch.org/}) and trained on NVIDIA Tesla V100 GPU.
$K$ is tuned within [1, 5, 10, 20].
Code will be released upon publication.

\begin{figure*}[t]
\centering
\begin{subfigure}[b]{.23\textwidth}
\includegraphics[width=\linewidth]{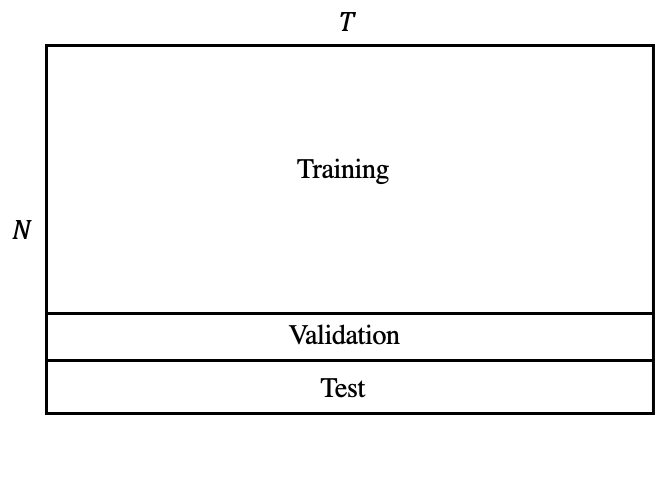}
 \caption{Single Imputation}\label{fig:single_impute}
\end{subfigure}\,
\begin{subfigure}[b]{.23\textwidth}
  \includegraphics[width=\linewidth]{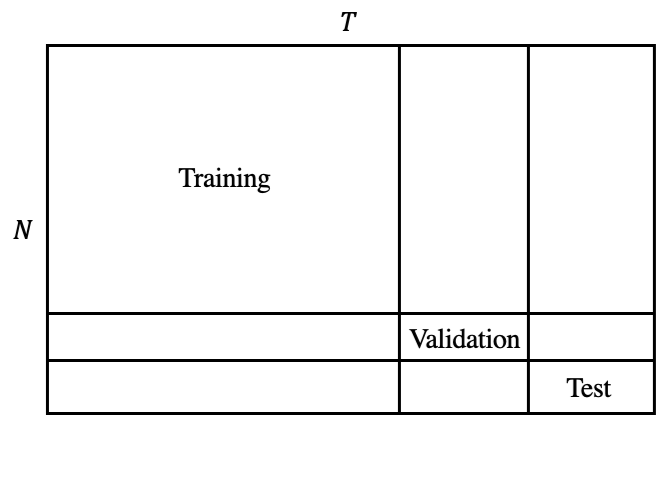}
  \caption{Single Forecasting}\label{fig:single_forecast}
\end{subfigure}\,
\begin{subfigure}[b]{.23\textwidth}
  \includegraphics[width=\linewidth]{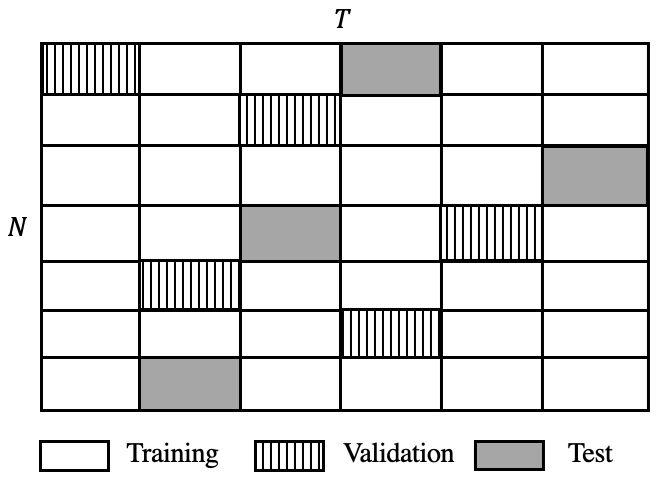}
  \caption{Networked Imputation}\label{fig:network_impute}
\end{subfigure}\,
\begin{subfigure}[b]{.23\textwidth}
  \includegraphics[width=\linewidth]{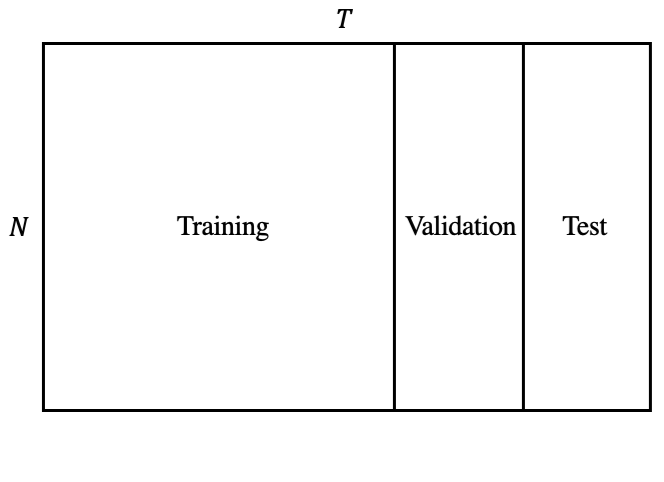}
  \caption{Networked Forecasting}\label{fig:network_forecast}
\end{subfigure}
\caption{Illustration of data splits.}
\label{fig:splits}
\end{figure*}

\begin{figure*}[t]
\centering
\begin{subfigure}[b]{.23\textwidth}
\includegraphics[width=\linewidth]{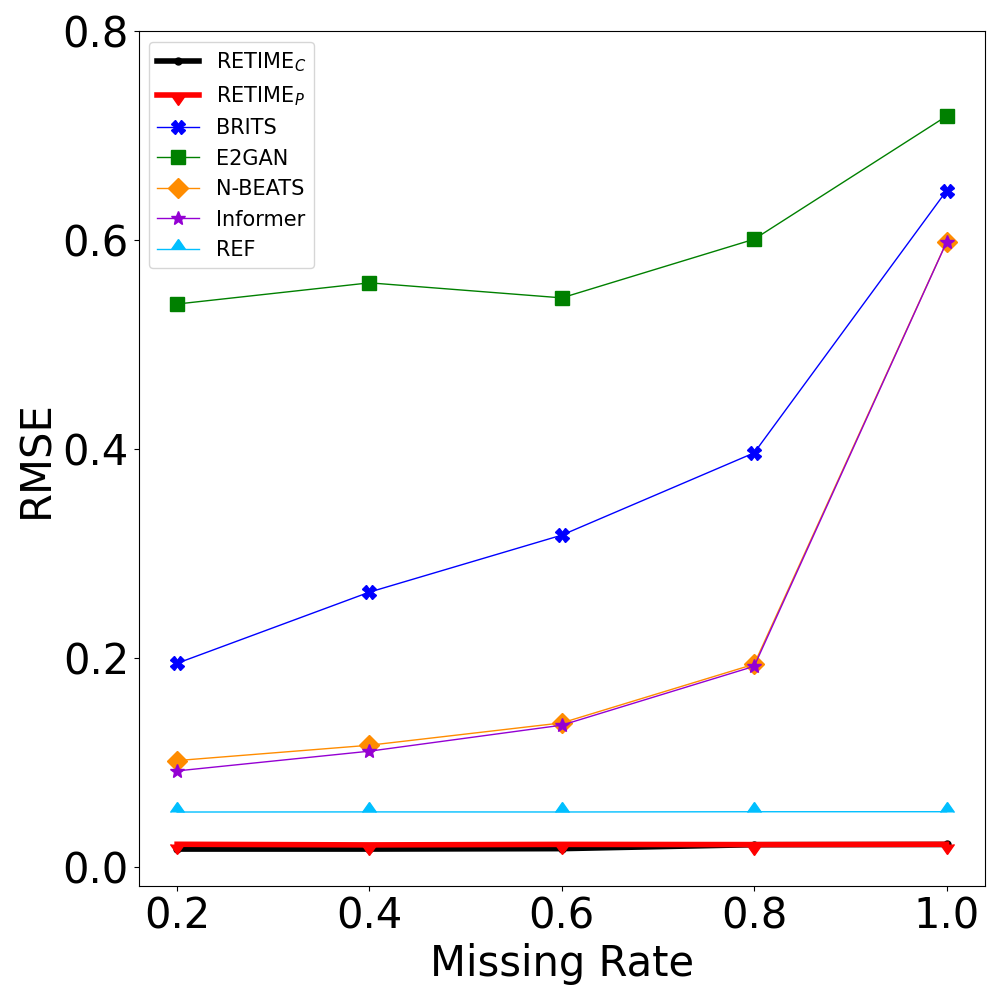}
 \caption{Single Imputation}\label{fig:single_impute_noaa}
\end{subfigure}\,
\begin{subfigure}[b]{.23\textwidth}
  \includegraphics[width=\linewidth]{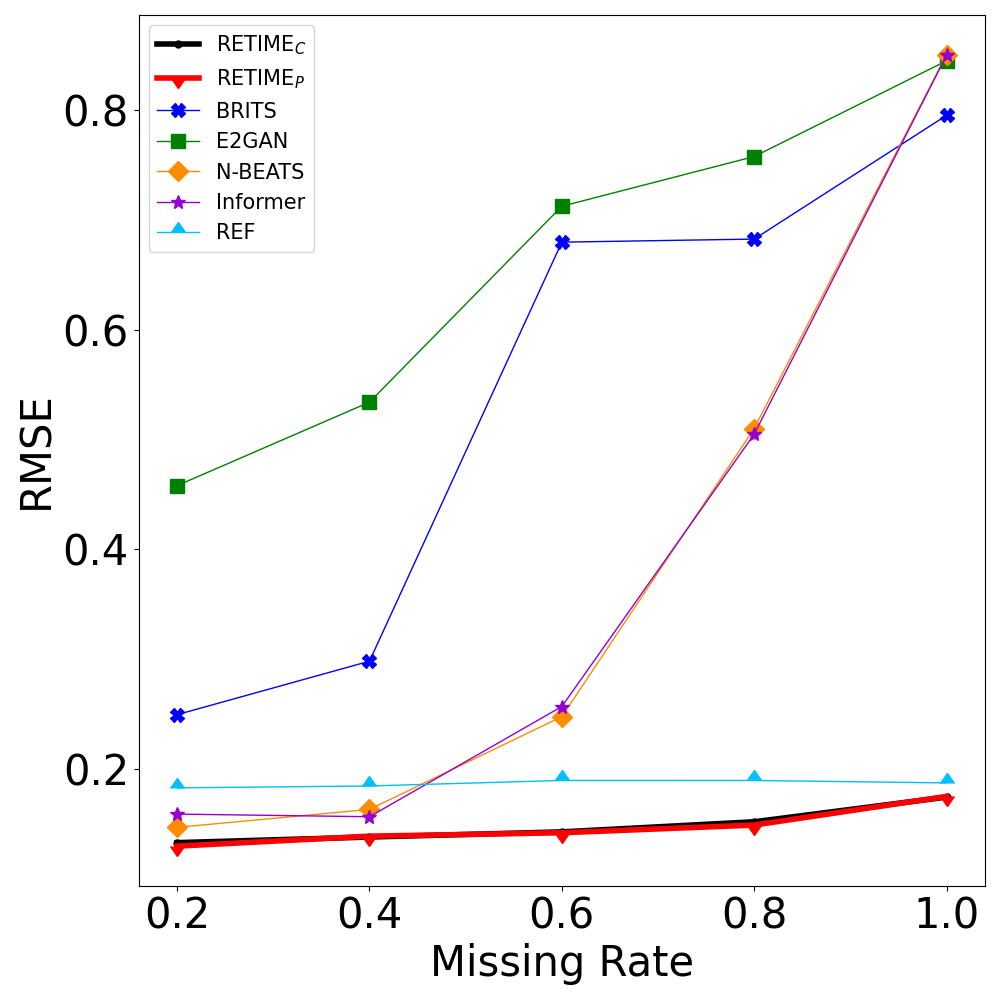}
  \caption{Single Forecasting}\label{fig:single_forecast_noaa}
\end{subfigure}\,
\begin{subfigure}[b]{.23\textwidth}
  \includegraphics[width=\linewidth]{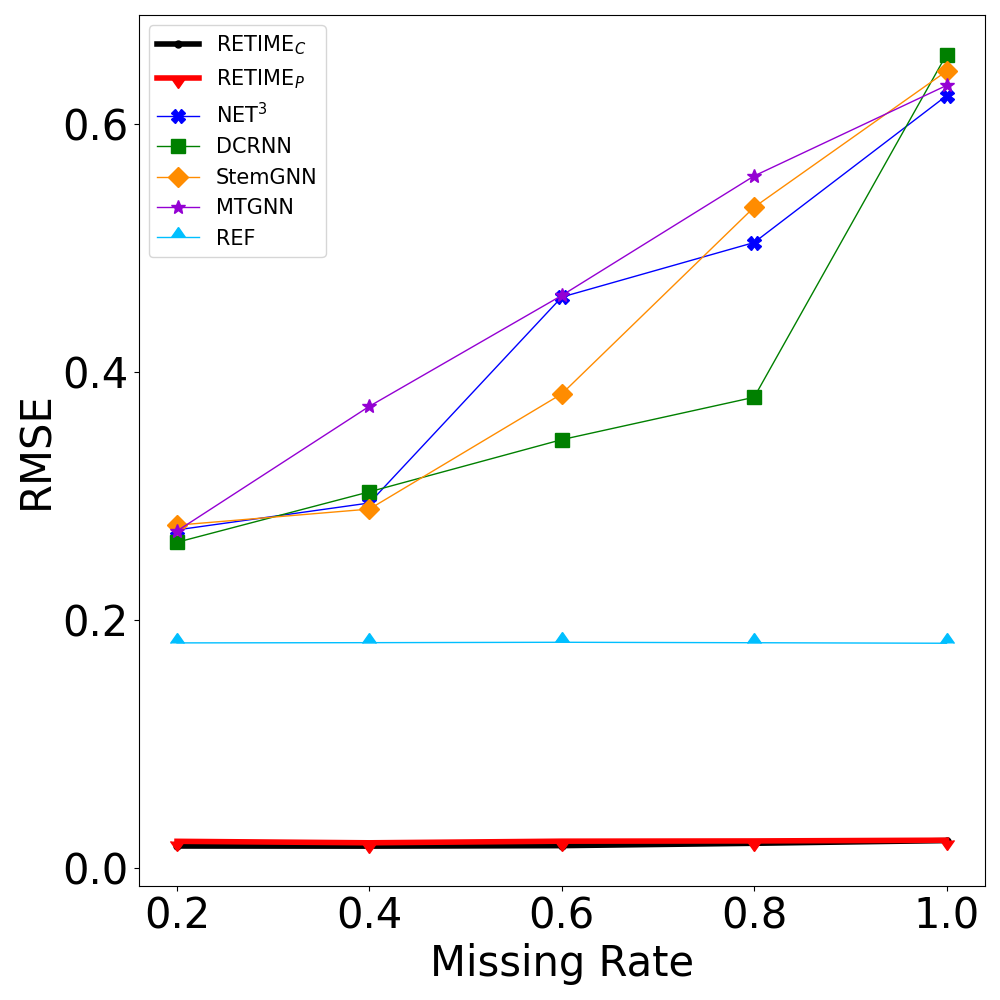}
  \caption{Networked Imputation}\label{fig:co_impute_noaa}
\end{subfigure}\,
\begin{subfigure}[b]{.23\textwidth}
  \includegraphics[width=\linewidth]{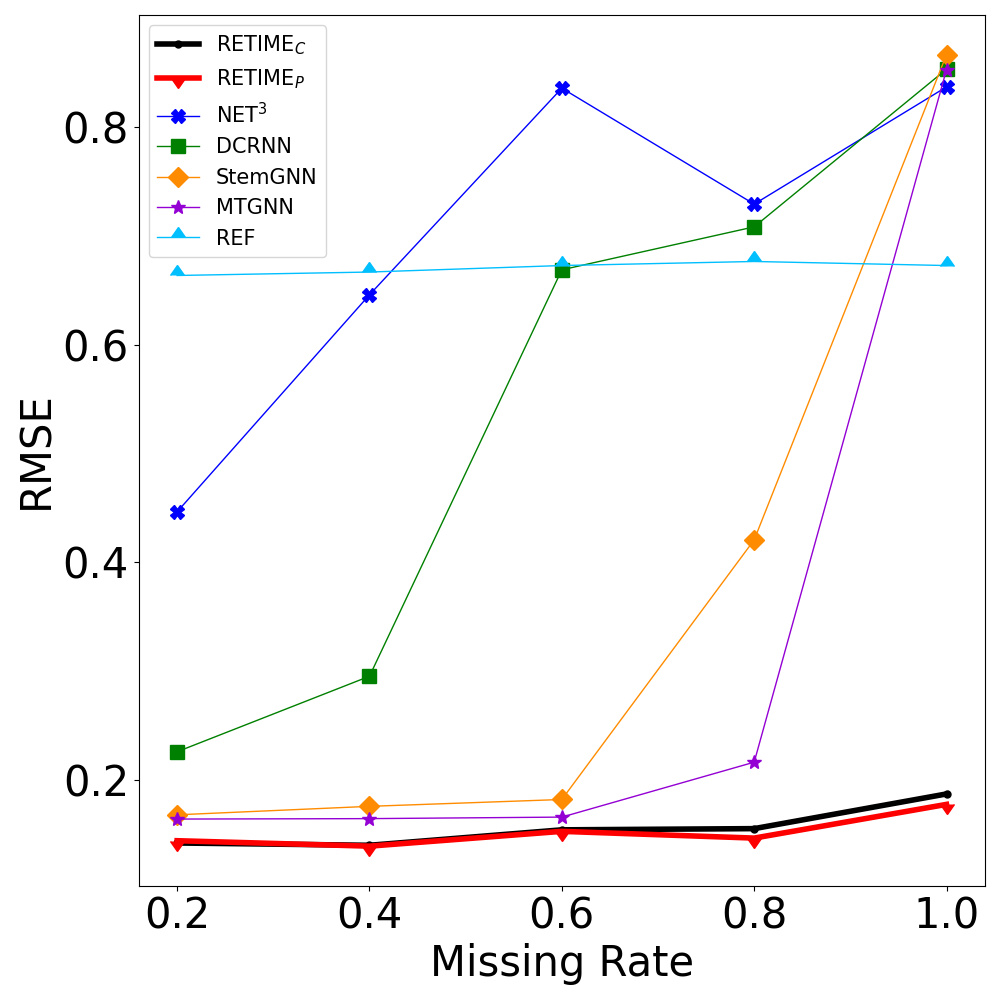}
  \caption{Networked Forecasting}\label{fig:co_forecast_noaa}
\end{subfigure}
\caption{MAE scores on the temperature dataset. The lower the better.}
\label{fig:noaa_mae}
\end{figure*}

\begin{figure}
    \centering
    \includegraphics[width=.4\textwidth]{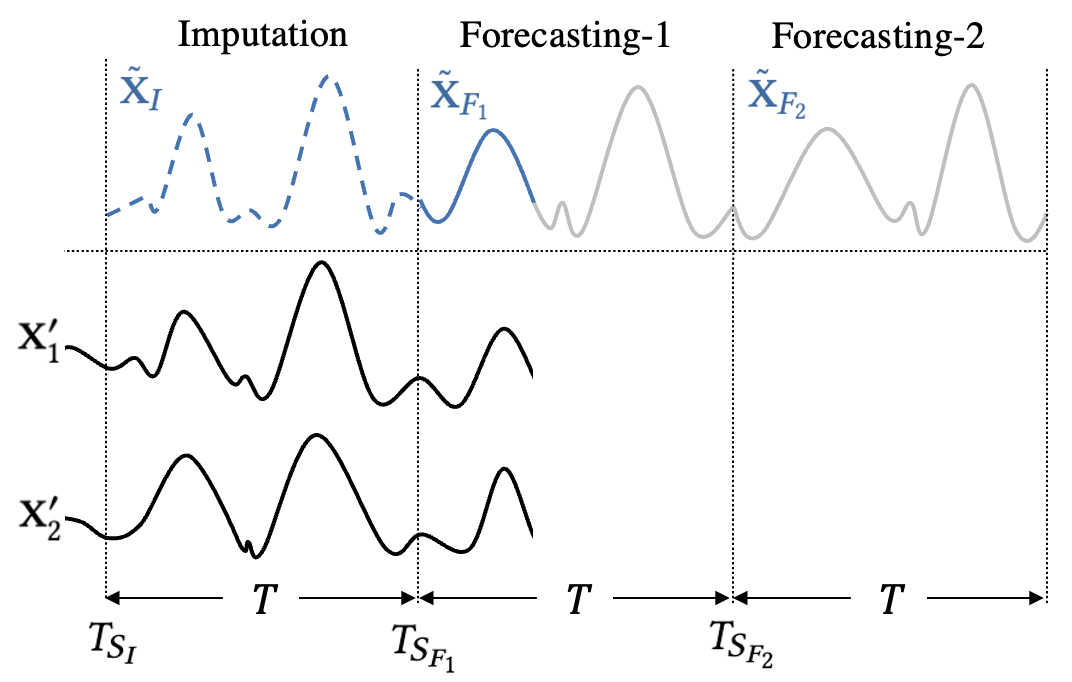}
    \caption{Illustration for selecting start time for different situations. The dashed curve has missing values. The grey curves are the future values to be predicted. $T_{S_I}$, $T_{S_{F_1}}$ and $T_{S_{F_2}}$ are the start times of the target snippets $\Tilde{\mathbf{X}}_I$, $\Tilde{\mathbf{X}}_{F_1}$ and $\Tilde{\mathbf{X}}_{F_2}$.}
    \label{fig:select_time}
\end{figure}

\section{Data Splits}\label{appendix:splits}
In Figure \ref{fig:splits}, we provide illustrations of data splits for different settings, where $N$ and $T$ are the numbers of time series and time steps.
In general, for single time series generation, given $N$ time series, we randomly select 10\%/10\% time series for validation and test.
For networked time series generation, we select 10\%/10\% \textit{snippets} from the entire datasets for validation/test. 

\section{Time Span Selection for References}\label{appendix:time_selection}
Instead of using the entire $\mathbf{X}'_k$ as a reference, we only use a snippet of it, since using the entire $\mathbf{X}'_k$ could introduce much irrelevant noisy information.
In fact, the total length of the reference $\mathbf{X}'_k\in\mathbb{R}^{T^d\times V}$ is much longer than the target $\Tilde{\mathbf{X}}\in\mathbb{R}^{T\times V}$: $T^d \gg T$, and the start time of $\mathbf{X}'_k$ is much earlier than $\Tilde{\mathbf{X}}$: $T_S^d\ll T_S$. 
Therefore, it is of necessity to select an appropriate time span for $\mathbf{X}_k'$, i.e. the start time $T_S'$ and length $T'$.
For simplicity, we fix $T'=T$, and thus the only hyper-parameter we need to determine is the start time $T_S'$.
Figure \ref{fig:select_time} provides an illustration for selecting the start time for different situations.
For imputation, we set $T_S'=T_S$, since it usually produces the best results in practice.
For forecasting, we either use $T_S'=T_S$ or a prior time $T_S'<T_S$.
There are two scenarios when a prior start time is necessary. 
The first one is when the time series has a clear periodic pattern, such as traffic occupancy. 
As illustrated by ``Forecasting-1" in Figure \ref{fig:select_time}, the data in the last period provides strong evidence for what will happen in the current period. 
The second one is when the database has no record after $T_S$, we have to resort to the historical data, which is illustrated by ``Forecasting-2" in Figure \ref{fig:select_time}.

\section{MAE Results on Temperature}
We present the Mean Absolute Error (MAE) scores on the the temperature dataset in Figure \ref{fig:noaa_mae}.
Comparing MAE scores in Figure \ref{fig:noaa_mae} and the RMSE scores on the temperature dataset in Figure \ref{fig:main_single}-\ref{fig:main_co}, we can observe that the relative performance of different methods are similar on RMSE and MAE.
